# Supplementary material for: Statistical biases in measurements with multiple candidates
Source: arXiv:1703.01128 ancillary file (2019-08-21)
Supplement: Supplementary file 1 [file Ancillary.pdf]

# Mathematical Details

This appendix contains additional material which will be removed from the paper.

The uncertainties on the $B$ yield are:

$$
\begin{aligned}
\sigma\left(\left\langle N^{\text{fit}}_{B^0}\right\rangle\right)^{\text{random}} &= \sqrt{\left\langle N^{\text{fit}}_{B^0}\right\rangle^{\text{random}} + \alpha\left(\frac{1}{2}N^{\text{gen}}_{\text{bkg}\,B^0}\mathcal{P}^{B^0}_{\text{bkg}} + \frac{1}{2}N^{\text{gen}}_{B^0}\mathcal{P}^{B^0}_{\text{sig}} + N^{\text{gen}}_{B^0}\right)} \\
\sigma\left(\left\langle N^{\text{fit}}_{B^0}\right\rangle\right)^{\text{all}} &= \sqrt{N^{\text{gen}}_{B^0} + \alpha\left(N^{\text{gen}}_{B^0}\mathcal{P}^{B^0}_{\text{sig}} + N^{\text{gen}}_{\text{bkg}\,B^0}\left(1+\mathcal{P}^{B^0}_{\text{bkg}}\right)\right)}.
\end{aligned}
$$

The uncertainties on $A_{\text{raw}}$ are:

$$
\begin{aligned}
\sigma(A)^{\text{all}}_{\text{raw}} =& \frac{2}{\left(N^{\text{gen}}_{\overline{B}^0} + N^{\text{gen}}_{B^0}\right)^2}\Bigg[N^{\text{gen}\,2}_{\overline{B}^0}\left(N^{\text{gen}}_{B^0} + \alpha\left(N^{\text{gen}}_{\text{bkg}\,B^0}\mathcal{P}^{B^0}_{\text{bkg}} + N^{\text{gen}}_{\text{bkg}\,B^0} + N^{\text{gen}}_{B^0}\mathcal{P}^{B^0}_{\text{sig}}\right)\right) \\
&+ N^{\text{gen}\,2}_{B^0}\left(N^{\text{gen}}_{\overline{B}^0} + \alpha\left(N^{\text{gen}}_{\text{bkg}\,\overline{B}^0}\mathcal{P}^{\overline{B}^0}_{\text{bkg}} + N^{\text{gen}}_{\text{bkg}\,\overline{B}^0} + N^{\text{gen}}_{\overline{B}^0}\mathcal{P}^{\overline{B}^0}_{\text{sig}}\right)\right)\Bigg]^{\frac{1}{2}} \\
\overset{N^{\text{gen}}_{B^0}=N^{\text{gen}}_{\overline{B}^0}}{=}& \frac{1}{2N^{\text{gen}\,2}_{B^0}}\Bigg[N^{\text{gen}\,2}_{B^0}\left(2N^{\text{gen}}_{B^0} + \alpha\left(N^{\text{gen}}_{\text{bkg}\,B^0}\mathcal{P}^{\overline{B}^0}_{\text{bkg}} + N^{\text{gen}}_{\text{bkg}\,B^0} + N^{\text{gen}}_{B^0}\mathcal{P}^{\overline{B}^0}_{\text{sig}}\right)\right. \\
&+ \left.\alpha\left(N^{\text{gen}}_{\text{bkg}\,B^0}\mathcal{P}^{B^0}_{\text{bkg}} + N^{\text{gen}}_{\text{bkg}\,B^0} + N^{\text{gen}}_{B^0}\mathcal{P}^{B^0}_{\text{sig}}\right)\right)\Bigg]^{\frac{1}{2}} \\
\sigma(A)^{\text{random}}_{\text{raw}} =& \frac{2}{\left(\frac{1}{2}N^{\text{gen}}_{\overline{B}^0}\mathcal{P}^{\overline{B}^0}_{\text{sig}} - N^{\text{gen}}_{\overline{B}^0} + \frac{1}{2}N^{\text{gen}}_{B^0}\mathcal{P}^{B^0}_{\text{sig}} - N^{\text{gen}}_{B^0}\right)^2}\Bigg[-N^{\text{gen}\,2}_{\overline{B}^0}\left(\frac{1}{2}\mathcal{P}^{\overline{B}^0}_{\text{sig}} - 1\right)^2 \\
&\left(\frac{1}{2}N^{\text{gen}}_{B^0}\mathcal{P}^{B^0}_{\text{sig}} - N^{\text{gen}}_{B^0} - \alpha\left(\frac{1}{2}N^{\text{gen}}_{\text{bkg}\,B^0}\mathcal{P}^{B^0}_{\text{bkg}} + \frac{1}{2}N^{\text{gen}}_{B^0}\mathcal{P}^{B^0}_{\text{sig}} + N^{\text{gen}}_{B^0}\right)\right) \\
&- N^{\text{gen}\,2}_{B^0}\left(\frac{1}{2}\mathcal{P}^{B^0}_{\text{sig}} - 1\right)^2\left(\frac{1}{2}N^{\text{gen}}_{\overline{B}^0}\mathcal{P}^{\overline{B}^0}_{\text{sig}} - N^{\text{gen}}_{\overline{B}^0}\right. \\
&- \left.\alpha\left(\frac{1}{2}N^{\text{gen}}_{\text{bkg}\,\overline{B}^0}\mathcal{P}^{\overline{B}^0}_{\text{bkg}} + \frac{1}{2}N^{\text{gen}}_{\overline{B}^0}\mathcal{P}^{\overline{B}^0}_{\text{sig}} + N^{\text{gen}}_{\overline{B}^0}\right)\right)\Bigg]^{\frac{1}{2}} \\
\overset{N^{\text{gen}}_{B^0}=N^{\text{gen}}_{\overline{B}^0}}{=}& \frac{2}{N^{\text{gen}\,2}_{B^0}\left(\frac{1}{2}\mathcal{P}^{\overline{B}^0}_{\text{sig}} + \frac{1}{2}\mathcal{P}^{B^0}_{\text{sig}} - 2\right)^2}\Bigg[N^{\text{gen}\,2}_{B^0}\left(-\left(\frac{1}{2}\mathcal{P}^{\overline{B}^0}_{\text{sig}} - 1\right)^2\left(\frac{1}{2}N^{\text{gen}}_{B^0}\mathcal{P}^{B^0}_{\text{sig}} - N^{\text{gen}}_{B^0}\right.\right. \\
&- \left.\alpha\left(\frac{1}{2}N^{\text{gen}}_{\text{bkg}\,B^0}\mathcal{P}^{B^0}_{\text{bkg}} + \frac{1}{2}N^{\text{gen}}_{B^0}\mathcal{P}^{B^0}_{\text{sig}} + N^{\text{gen}}_{B^0}\right)\right) - \left(\frac{1}{2}\mathcal{P}^{B^0}_{\text{sig}} - 1\right)^2\left(\frac{1}{2}N^{\text{gen}}_{B^0}\mathcal{P}^{\overline{B}^0}_{\text{sig}}\right. \\
&- \left.\left.N^{\text{gen}}_{B^0} - \alpha\left(\frac{1}{2}N^{\text{gen}}_{\text{bkg}\,B^0}\mathcal{P}^{\overline{B}^0}_{\text{bkg}} + \frac{1}{2}N^{\text{gen}}_{B^0}\mathcal{P}^{\overline{B}^0}_{\text{sig}} + N^{\text{gen}}_{B^0}\right)\right)\right)\Bigg]^{\frac{1}{2}}.
\end{aligned}
$$

For large values of $\eta^{B^0}_{\text{best}}$, the arbitration method achieves a smaller relative uncertainty on the $B$ yield than taking all candidates, as seen in Fig. 4. The crossing-point value of $\eta^{B^0}_{\text{best}}$ is

determined as follows. The fitted parameters for the all method are

$$\left(N_{B^0}^{\text{fit}}\right)_{\text{all}} = N_{B^0}^{\text{gen}}$$
$$\sigma\left(N_{B^0}^{\text{fit}}\right)_{\text{all}} = \sqrt{N_{B^0}^{\text{gen}} + \alpha\left[N_{\text{bkg}\,B^0}^{\text{gen}} + \mathcal{P}_{\text{sig}}^{B^0} N_{B^0}^{\text{gen}} + \mathcal{P}_{\text{bkg}}^{B^0} N_{\text{bkg}\,B^0}^{\text{gen}}\right]}.$$

For the random selection

$$\left(N_{B^0}^{\text{fit}}\right)_{\text{random}} = N_{B^0}^{\text{gen}} - \frac{1}{2} N_{B^0}^{\text{gen}} \mathcal{P}_{\text{sig}}^{B^0}$$
$$\sigma\left(N_{B^0}^{\text{fit}}\right)_{\text{random}} = \sqrt{\left(N_{B^0}^{\text{fit}}\right)_{\text{random}} + \alpha\left[N_{\text{bkg}\,B^0}^{\text{gen}} + \frac{1}{2}\left(\mathcal{P}_{\text{sig}}^{B^0} N_{B^0}^{\text{gen}} + \mathcal{P}_{\text{bkg}}^{B^0} N_{\text{bkg}\,B^0}^{\text{gen}}\right)\right]}.$$

This is just a special case of best selection, for which we have

$$\left(N_{B^0}^{\text{fit}}\right)_{\text{best}} = N_{B^0}^{\text{gen}} - (1-\eta_{\text{best}}^{B^0}) N_{B^0}^{\text{gen}} \mathcal{P}_{\text{sig}}^{B^0}$$
$$\sigma\left(N_{B^0}^{\text{fit}}\right)_{\text{best}} = \sqrt{\left(N_{B^0}^{\text{fit}}\right)_{\text{best}} + \alpha\left[N_{\text{bkg}\,B^0}^{\text{gen}} + (1-\eta_{\text{best}}^{B^0})\left(\mathcal{P}_{\text{sig}}^{B^0} N_{B^0}^{\text{gen}} + \mathcal{P}_{\text{bkg}}^{B^0} N_{\text{bkg}\,B^0}^{\text{gen}}\right)\right]}.$$

The relative uncertainty is

$$\frac{\sigma\left(N_{B^0}^{\text{fit}}\right)_{\text{best}}}{\left(N_{B^0}^{\text{fit}}\right)_{\text{best}}} = \frac{\sqrt{\left(N_{B^0}^{\text{fit}}\right)_{\text{best}} + \alpha\left[N_{\text{bkg}\,B^0}^{\text{gen}} + (1-\eta_{\text{best}}^{B^0})\left(\mathcal{P}_{\text{sig}}^{B^0} N_{B^0}^{\text{gen}} + \mathcal{P}_{\text{bkg}}^{B^0} N_{\text{bkg}\,B^0}^{\text{gen}}\right)\right]}}{N_{B^0}^{\text{gen}} - (1-\eta_{\text{best}}^{B^0}) N_{B^0}^{\text{gen}} \mathcal{P}_{\text{sig}}^{B^0}}.$$

At some point this becomes smaller than the relative uncertainty for the all case

$$\frac{\sigma\left(N_{B^0}^{\text{fit}}\right)_{\text{all}}}{\left(N_{B^0}^{\text{fit}}\right)_{\text{all}}} = \frac{\sqrt{N_{B^0}^{\text{gen}} + \alpha\left[N_{\text{bkg}\,B^0}^{\text{gen}} + \mathcal{P}_{\text{sig}}^{B^0} N_{B^0}^{\text{gen}} + \mathcal{P}_{\text{bkg}}^{B^0} N_{\text{bkg}\,B^0}^{\text{gen}}\right]}}{N_{B^0}^{\text{gen}}},$$

which is a quadratic equation to be solved for $\eta_{\text{best}}^{B^0}$. It has solutions if

$$\begin{aligned}
&4{N_{\text{bkg}\,B^0}^{\text{gen}}}^2 {\mathcal{P}_{\text{bkg}}^{B^0}}^2 \mathcal{P}_{\text{sig}}^{B^0} \alpha^2 + {N_{\text{bkg}\,B^0}^{\text{gen}}}^2 {\mathcal{P}_{\text{bkg}}^{B^0}}^2 \alpha^2 + 4{N_{\text{bkg}\,B^0}^{\text{gen}}}^2 \mathcal{P}_{\text{bkg}}^{B^0} \mathcal{P}_{\text{sig}}^{B^0} \alpha^2 \\
&\quad + 12 N_{\text{bkg}\,B^0}^{\text{gen}} N_{B^0}^{\text{gen}} \mathcal{P}_{\text{bkg}}^{B^0} {\mathcal{P}_{\text{sig}}^{B^0}}^2 \alpha^2 + 2 N_{\text{bkg}\,B^0}^{\text{gen}} N_{B^0}^{\text{gen}} \mathcal{P}_{\text{bkg}}^{B^0} \mathcal{P}_{\text{sig}}^{B^0} \alpha^2 \\
&+ 2 N_{\text{bkg}\,B^0}^{\text{gen}} N_{B^0}^{\text{gen}} \mathcal{P}_{\text{bkg}}^{B^0} \mathcal{P}_{\text{sig}}^{B^0} \alpha + 8 N_{\text{bkg}\,B^0}^{\text{gen}} N_{B^0}^{\text{gen}} {\mathcal{P}_{\text{sig}}^{B^0}}^2 \alpha^2 + 8 N_{B^0}^{\text{gen}2} {\mathcal{P}_{\text{sig}}^{B^0}}^3 \alpha^2 \\
&\quad + N_{B^0}^{\text{gen}2} {\mathcal{P}_{\text{sig}}^{B^0}}^2 \alpha^2 + 6 N_{B^0}^{\text{gen}2} {\mathcal{P}_{\text{sig}}^{B^0}}^2 \alpha + N_{B^0}^{\text{gen}2} {\mathcal{P}_{\text{sig}}^{B^0}}^2 > 0,
\end{aligned}$$

which is the case here. One solution is negative and the correct is

$$
\begin{aligned}
\eta^{B^0}_{\text{best}}(\text{cross}) =& \frac{1}{N^{\text{gen}\,2}_{B^0}\mathcal{P}^{B^0\,2}_{\text{sig}}\left(N^{\text{gen}}_{\text{bkg}\;B^0}\mathcal{P}^{B^0}_{\text{bkg}}\alpha + N^{\text{gen}}_{\text{bkg}\;B^0}\alpha + N^{\text{gen}}_{B^0}\mathcal{P}^{B^0}_{\text{sig}}\alpha + N^{\text{gen}}_{B^0}\right)} \\
& \Bigg( N^{\text{gen}}_{\text{bkg}\;B^0}N^{\text{gen}\,2}_{B^0}\mathcal{P}^{B^0}_{\text{bkg}}\mathcal{P}^{B^0\,2}_{\text{sig}}\alpha - N^{\text{gen}}_{\text{bkg}\;B^0}N^{\text{gen}\,2}_{B^0}\mathcal{P}^{B^0}_{\text{bkg}}\mathcal{P}^{B^0}_{\text{sig}}\alpha \\
& - \frac{N^{\text{gen}}_{\text{bkg}\;B^0}\mathcal{P}^{B^0}_{\text{bkg}}}{2}N^{\text{gen}\,2}_{B^0}\alpha + N^{\text{gen}}_{\text{bkg}\;B^0}N^{\text{gen}\,2}_{B^0}\mathcal{P}^{B^0\,2}_{\text{sig}}\alpha - N^{\text{gen}}_{\text{bkg}\;B^0}N^{\text{gen}\,2}_{B^0}\mathcal{P}^{B^0}_{\text{sig}}\alpha \\
& + N^{\text{gen}\,3}_{B^0}\mathcal{P}^{B^0\,3}_{\text{sig}}\alpha - N^{\text{gen}\,3}_{B^0}\mathcal{P}^{B^0\,2}_{\text{sig}}\alpha + N^{\text{gen}\,3}_{B^0}\mathcal{P}^{B^0\,2}_{\text{sig}} - \frac{\mathcal{P}^{B^0}_{\text{sig}}\alpha}{2}N^{\text{gen}\,3}_{B^0} - \frac{N^{\text{gen}\,3}_{B^0}\mathcal{P}^{B^0}_{\text{sig}}}{2} \\
& + \frac{1}{2}\Bigg[ N^{\text{gen}\,4}_{B^0}\Bigg( 4N^{\text{gen}}_{\text{bkg}\;B^0}{}^{2}\mathcal{P}^{B^0\,2}_{\text{bkg}}\mathcal{P}^{B^0}_{\text{sig}}\alpha^2 + N^{\text{gen}}_{\text{bkg}\;B^0}{}^{2}\mathcal{P}^{B^0\,2}_{\text{bkg}}\alpha^2 + 4N^{\text{gen}}_{\text{bkg}\;B^0}{}^{2}\mathcal{P}^{B^0}_{\text{bkg}}\mathcal{P}^{B^0}_{\text{sig}}\alpha^2 \\
& + 12N^{\text{gen}}_{\text{bkg}\;B^0}N^{\text{gen}}_{B^0}\mathcal{P}^{B^0}_{\text{bkg}}\mathcal{P}^{B^0\,2}_{\text{sig}}\alpha^2 + 2N^{\text{gen}}_{\text{bkg}\;B^0}N^{\text{gen}}_{B^0}\mathcal{P}^{B^0}_{\text{bkg}}\mathcal{P}^{B^0}_{\text{sig}}\alpha^2 \\
& + 2N^{\text{gen}}_{\text{bkg}\;B^0}N^{\text{gen}}_{B^0}\mathcal{P}^{B^0}_{\text{bkg}}\mathcal{P}^{B^0}_{\text{sig}}\alpha + 8N^{\text{gen}}_{\text{bkg}\;B^0}N^{\text{gen}}_{B^0}\mathcal{P}^{B^0\,2}_{\text{sig}}\alpha^2 + 8N^{\text{gen}\,2}_{B^0}\mathcal{P}^{B^0\,3}_{\text{sig}}\alpha^2 \\
& + N^{\text{gen}\,2}_{B^0}\mathcal{P}^{B^0\,2}_{\text{sig}}\alpha^2 + 6N^{\text{gen}\,2}_{B^0}\mathcal{P}^{B^0\,2}_{\text{sig}}\alpha + N^{\text{gen}\,2}_{B^0}\mathcal{P}^{B^0\,2}_{\text{sig}}\Bigg)\Bigg]^{\frac{1}{2}}\Bigg).
\end{aligned}
$$

With the default values $N^{\text{gen}}_{B^0} = 50000$, $N^{\text{gen}}_{\text{bkg}\;B^0} = 50000$, $\mathcal{P}^{B^0}_{\text{sig}} = 0.2$, $\mathcal{P}^{B^0}_{\text{bkg}} = 0.2$, $\alpha = 0.2334$, the result is $\eta^{B^0}_{\text{best}}(\text{cross}) = 0.77$, as can be read from Fig. 4.
